# Supplementary material for: Stylized Face Sketch Extraction via Generative Prior with Limited Data
Source: arXiv:2403.11263 source file (2024-03-17)
Supplement: Supplementary file 1 [file 89_appendix.tex]

\begin{table*}[t]
\centering
\scriptsize % reduce font size
\setlength{\tabcolsep}{2pt} % reduce column spacing
 % increase row height
\begin{tabular}{c|cc|cc|cc|cc|cc|cc|cc|cc}
\textbf{Methods} & \multicolumn{2}{c|}{\textbf{Style 1}} & \multicolumn{2}{c|}{\textbf{Style 2}} & \multicolumn{2}{c|}{\textbf{Style 3}} & \multicolumn{2}{c|}{\textbf{Style 4}} & \multicolumn{2}{c|}{\textbf{Style 5}} & \multicolumn{2}{c|}{\textbf{Style 6}}& \multicolumn{2}{c|}{\textbf{Style 7}}& \multicolumn{2}{c}{\textbf{Average}} \\
\cline{2-17}
& LPIPS & FID & LPIPS & FID & LPIPS & FID & LPIPS & FID & LPIPS & FID & LPIPS & FID & LPIPS & FID & LPIPS & FID \\
\hline
Ours & 0.215 & 66.968 & 0.203 & 80.500 & 0.234 & 73.060 & 0.187 & 93.458 & 0.152 & 88.242 & 0.174 & 65.692 & 0.155 & 134.109 & 0.188 & 86.004 \\
Wo l1 & 0.230 & 80.846 & 0.207 & 85.862 & 0.244 & 84.659 & 0.188 & 83.762 & 0.177 & 87.591 & 0.166 & 70.577 & 0.161 & 211.528 & 0.196 & 100.689 \\
W l1 & 0.231 & 95.680 & 0.219 & 109.351 & 0.264 & 124.294 & 0.191 & 122.911 & 0.173 & 110.680 & 0.184 & 104.264 & 0.152 & 181.034 & 0.202 & 121.173 \\
Wo att & 0.220 & 71.826 & 0.200 & 76.171 & 0.235 & 80.380 & 0.188 & 86.525 & 0.160 & 90.182 & 0.179 & 73.188 & 0.157 & 170.026 & 0.191 & 92.614 \\
Wo clip & 0.230 & 80.746 & 0.201 & 71.541 & 0.252 & 78.875 & 0.191 & 96.546 & 0.173 & 137.266 & 0.183 & 72.654 & 0.160 & 173.079 & 0.199 & 101.529 \\
\end{tabular}
\end{table*}

\begin{table*}[t]
\centering
\scriptsize % reduce font size
\setlength{\tabcolsep}{2pt} % reduce column spacing
 % increase row height
\begin{tabular}{c|cc|cc|cc|cc|cc|cc|cc|cc|}
\textbf{Number of data} & \multicolumn{2}{c|}{\textbf{Style 1}} & \multicolumn{2}{c|}{\textbf{Style 2}} & \multicolumn{2}{c|}{\textbf{Style 3}} & \multicolumn{2}{c|}{\textbf{Style 4}} & \multicolumn{2}{c|}{\textbf{Style 5}} & \multicolumn{2}{c|}{\textbf{Style 6}}& \multicolumn{2}{c|}{\textbf{Style 7}}& \multicolumn{2}{c|}{\textbf{Average}} \\
\cline{2-17}
& LPIPS & FID & LPIPS & FID & LPIPS & FID & LPIPS & FID & LPIPS & FID & LPIPS & FID & LPIPS & FID & LPIPS & FID \\
\hline
4 & 0.252 & 151.216 & 0.234 & 177.718 & 0.287 & 186.108 & 0.198 & 182.863 & 0.178 & 125.366 & 0.182 & 112.242 & 0.162 & 220.742 & 0.213 & 165.179 \\
8 & 0.225 & 87.336 & 0.211 & 107.074 & 0.257 & 104.057 & 0.189 & 125.257 & 0.175 & 106.560 & 0.183 & 78.375 & 0.157 & 206.584 & 0.199 & 116.463 \\
16 & 0.215 & 66.968 & 0.203 & 80.500 & 0.234 & 73.060 & 0.187 & 93.458 & 0.152 & 88.242 & 0.174 & 65.692 & 0.155 & 134.109 & 0.188 & 86.004 \\
24 & 0.214 & 68.093 & 0.196 & 60.510 & 0.224 & 67.676 & 0.179 & 68.992 & 0.178 & 77.352 & 0.175 & 65.850 & 0.152 & 160.824 & 0.188 & 81.328 \\
32 & 0.211 & 67.320 & 0.193 & 61.606 & 0.223 & 66.876 & 0.180 & 58.006 & 0.147 & 74.973 & 0.174 & 66.568 & 0.151 & 158.978 & 0.183 & 79.190 \\
\end{tabular}
\end{table*}

\begin{table*}[t]
\centering
\scriptsize % reduce font size
\setlength{\tabcolsep}{2pt} % reduce column spacing
 % increase row height
\caption{Quantitative results of comparison with baselines. The best LPIPS score is annotated in bold while FID best scores are underlined.} \vspace{-10pt}
%\resizebox{\textwidth}{!}{%
\begin{tabular}{|c|cccccccccc|}
\noalign{\smallskip}\noalign{\smallskip}\hline

\hline
Sketch styles & SKSF-A(style 1) & SKSF-A(style 2) & SKSF-A(style 3) & SKSF-A(style 4) & SKSF-A(style 5) & SKSF-A(style 6) & SKSF-A(style 7)           & APDrawing           & CUFS                  & AVERAGE            \\ \hline
    Methods      & \multicolumn{10}{c|}{\textbf{LPIPS↓}/\underline{FID}↓}                                                     \\ \hline
    
\textbf{Ours}                & \textbf{0.1669}/\underline{62.24} & 0.1552/90.12 & 0.1665/76.53 & \textbf{0.1405}/\underline{75.11} & 0.1956/175.68 & \textbf{0.1025}/86.54 & \textbf{0.1112}/149.01 & 0.2078/94.13 & 0.0513/91.54 & \textbf{0.1442}/100.10  \\ \hline 
Ref2sketch~\cite{ashtari2022reference}                & 0.1998/129.96 & \textbf{0.1595}/\underline{56.85} & 0.1828/80.58 & 0.1597/81.45 & 0.1836/\underline{141.48} & 0.1345/\underline{73.98} & 0.1423/\underline{143.15} & 0.2547/82.27 & 0.0735/106.83 & 0.1656/99.62 \\ 
\citet{chan2022learning} with full                & 0.2082/166.18 & 0.1795/127.41 & 0.1988/143.14 & 0.1753/161.79 & 0.2059/271.74 & 0.1520/162.97 & 0.1362/245.96 & 0.2685/145.70 & \textbf{0.0488}/\underline{71.46} & 0.1748/166.26 \\
\citet{yi2020unpaired} with full                & 0.1838/101.21 & 0.1529/70.15 & \textbf{0.1646}/\underline{72.04} & 0.1543/85.34 & \textbf{0.1696}/157.11 & 0.1177/77.73 & 0.1141/153.64 & \textbf{0.1809}/\textbf{62.41} & 0.0674/99.67 & 0.1450/\underline{97.70} \\
\hline
\citet{ojha2021few}                & 0.2487/138.63 & 0.2389/157.19 & 0.2393/116.46 & 0.2125/116.49 & 0.2570/204.09 & 0.1854/114.73 & 0.1400/229.58 & 0.2697/154.13 & 0.0911/160.73 & 0.2092/154.67 \\
\citet{chan2022learning} with limited                & 0.2212/260.91 & 0.2053/294.25 & 0.2218/311.29 & 0.1888/278.71 & 0.2217/353.55 & 0.1619/209.86 & 0.1436/277.72 & 0.2659/181.49 & 0.0577/78.36 & 0.1875/249.57 \\ 
\citet{yi2020unpaired} with limited                & 0.1945/125.09 & 0.1645/92.47 & 0.1782/116.77 & 0.1619/162.56 & 0.1838/189.84 & 0.1294/104.16 & 0.1220/182.46 & 0.2016/81.28 & 0.0518/82.62 & 0.1542/126.36 \\ 

\hline 
\end{tabular}%}
\label{Tab:baseline}
\end{table*}

\begin{table*}[t]
\centering
\scriptsize % reduce font size
\setlength{\tabcolsep}{2pt} % reduce column spacing
 % increase row height
\caption{Ablation study using LPIPS and FID scores.} \vspace{-10pt}
%\resizebox{\textwidth}{!}{%
\begin{tabular}{|c|cccccccccc|}
\noalign{\smallskip}\noalign{\smallskip}\hline

\hline
Sketch styles & SKSF-A(style 1) & SKSF-A(style 2) & SKSF-A(style 3) & SKSF-A(style 4) & SKSF-A(style 5) & SKSF-A(style 6) & SKSF-A(style 7)           & APDrawing           & CUFS                  & AVERAGE            \\ \hline
    Methods      & \multicolumn{10}{c|}{\textbf{LPIPS↓}/\underline{FID}↓}                                                     \\ \hline
    
\textbf{Ours} & \textbf{0.2155}/\underline{66.97} & \textbf{0.1868}/93.46 & 0.2029/80.50 & 0.1742/\underline{65.69} & \textbf{0.2341}/\underline{73.06} & \textbf{0.1524}/88.24 & 0.1551/\underline{134.11} & \textbf{0.2118}/\underline{87.05} & 0.0623/\underline{43.47} & \textbf{0.1772}/\underline{81.39} \\
Ours W/O $L_1 initialize$ & 0.2300/80.85 & 0.1876/\underline{83.76} & 0.2068/85.86 & \textbf{0.1658}/70.58 & 0.2442/84.66 & 0.1768/87.59 & 0.1612/211.53 & 0.2162/103.85 & 0.0648/46.12 & 0.1837/94.98 \\
Ours W $L_1$ (until the end) & 0.2308/95.68 & 0.1913/122.91 & 0.2194/109.35 & 0.1836/104.26 & 0.2641/124.29 & 0.1729/110.68 & \textbf{0.1524}/181.03 & 0.2190/126.98 & 0.0632/45.81 & 0.1885/113.45 \\
Ours W/O attention & 0.2197/71.83 & 0.1879/86.52 & \textbf{0.2004}/76.17 & 0.1785/73.19 & 0.2351/80.38 & 0.1599/90.18 & 0.1573/170.03 & 0.2233/141.53 & \textbf{0.0621}/45.34 & 0.1805/92.80 \\
Ours W one adversarial loss & 0.2329/80.75 & 0.1935/91.08 & 0.2048/79.80 & 0.1843/67.58 & 0.2444/93.23 & 0.1785/\underline{74.52} & 0.1552/204.05 & 0.2180/111.29 & 0.0632/44.23 & 0.1861/94.06 \\
Ours W/O $L_{clip}$ & 0.2296/89.17 & 0.1908/96.55 & 0.2010/\underline{71.54} & 0.1833/72.65 & 0.2524/78.88 & 0.1729/137.27 & 0.1605/173.08 & 0.2153/98.12 & 0.0636/46.80 & 0.1855/96.01 \\ 

\hline 
\end{tabular}%}
\label{Tab:baseline}
\end{table*}
